# Supplementary material for: Revisiting Backdoor Attacks against Large Vision-Language Models from Domain Shift
Source: arXiv:2406.18844 source file (2024-12-16)
Supplement: Supplementary file 2 [file TableAppendix-PR-Flickr.tex]

\begin{table*}[h]
    \centering
    \caption{Attack performance of different backdoor attacks with different poisoning rates under Flickr30K dataset}
    \label{tab:scalability_flickr}
    \resizebox{\textwidth}{!}{%
    \setlength{\tabcolsep}{10pt}
    
    \begin{tabular}{lccccccccccc}
        \toprule
        \multirow{2}{*}{Method} & \multirow{2}{*}{Char Change} & \multicolumn{2}{c}{0.1\%} & \multicolumn{2}{c}{0.5\%} & \multicolumn{2}{c}{1\%} & \multicolumn{2}{c}{5\%} & \multicolumn{2}{c}{10\%} \\ \cmidrule(r){3-4} \cmidrule(r){5-6} \cmidrule(r){7-8} \cmidrule(r){9-10} \cmidrule(r){11-12}
         &  & \multicolumn{1}{c}{ACC(\%)} & \multicolumn{1}{c}{ASR(\%)} & \multicolumn{1}{c}{ACC(\%)} & \multicolumn{1}{c}{ASR(\%)} & \multicolumn{1}{c}{ACC(\%)} & \multicolumn{1}{c}{ASR(\%)} & \multicolumn{1}{c}{ACC(\%)} & \multicolumn{1}{c}{ASR(\%)} & \multicolumn{1}{c}{ACC(\%)} & \multicolumn{1}{c}{ASR(\%)} \\ \midrule
        \cellcolor[HTML]{F1B9B6}AddSent & 12 & 43.62 & 0.00 & 45.13 & 0.00 & 48.50 & 29.53 & 48.27 & 25.57 & 48.51 & 29.57 \\
        \cellcolor[HTML]{F1B9B6}TextBadNets & 6 & 44.31 & 0.15 & 47.16 & 3.82 & 45.76 & 93.25 & 47.34 & 97.23 & 48.15 & 97.23 \\
        \cellcolor[HTML]{F1B9B6}$\text{TextBadNets}^{*}$ & 12 & 45.08 & 0.15 & 44.78 & 55.87 & 46.68 & 99.31 & 46.99 & 99.98 & 49.85 & 100.00 \\
        \cellcolor[HTML]{FEEBB8}StyleBkd & 6.7 & 46.15 & 0.24 & 48.17 & 100.00 & 47.65 & 100.00 & 49.43 & 100.00 & 49.74 & 100.00 \\
        \cellcolor[HTML]{D7E8F2}GCG & 6 & 46.09 & 1.22 & 47.30 & 100.00 & 47.72 & 99.48 & 46.95 & 100.00 & 50.40 & 100.00 \\
        \cellcolor[HTML]{D7E8F2}$\text{GCG}^{*}$ & 12 & 45.53 & 0.11 & 45.53 & 61.69 & 47.21 & 97.11 & 48.16 & 100.00 & 48.16 & 100.00 \\ 
        \bottomrule
    \end{tabular}%
}
\end{table*}
